# Supplementary material for: Persistent Homology via Ellipsoids
Source: arXiv:2408.11450 source file (2026-11-26)
Supplement: Supplementary file 1 [file appendix.tex]

\documentclass[../ellipsoid-main.tex]{subfiles}

\begin{document}

\subsection{PCA Ellipsoids and their Properties}
In the construction of ellipsoids we set the lengths of axes to be $\epsilon$ in tangent directions and $\frac{\epsilon}{q}$ in normal directions (See Definition~\ref{def:ellipsoid}). One may ask why we chose this particular axis scaling, since one could argue that the more natural choice would have been scaling the axes according to the sizes of the singular values. We show in this appendix that this construction is also stable, but did not perform as well in practice as will be shown below. 

We define the ellipsoid with PCA axes as follows.
\begin{definition}[PCA Ellipsoid]\label{def:pca-ellipsoid}
Let $x \in \RR^n$. We define the \emph{PCA ellipsoid} centered at $x$ with scale parameter $\varepsilon > 0$ by
\[
E^{\PCA}_\varepsilon(x) \coloneqq \bigl\{\, y \in \RR^n \;\big|\; (y - x)^\top \bigl( \mathbf N_n(x) \mathbf N_n(x)^\top \bigr)^{-1} (y - x) \le \varepsilon^2 \,\bigr\}.
\]
Let $X$ be a finite subset of $\RR^n$. We denote the Rips-type filtration of $X$ arising from PCA ellipsoid complexes (as in Definition~\ref{def:ellipsoid_complex}) by $E^{PCA}(X)$.
\end{definition}
Similarly to the case of Rips-type ellipsoid barcodes, PCA ellipsoid barcodes also satisfy a stability theorem.

\begin{theorem}\label{thm:PCA_stability}
Let $X \subset \RR^n$ be an $n$-generic subset (Definition~\ref{def:genericity}), and let \(\mathfrak{p}\colon X \to \RR^n\) be a \(\delta\)-perturbation with \(\delta \in [0, \delta_0)\) for some \(\delta_0 > 0\). Then
\[
\distance_b\bigl(\dgm(E^{\PCA}(X)),\, \dgm(E^{\PCA}(\mathfrak{p}(X)))\bigr)
    \le C\delta = C\,\distance_H(X, \mathfrak{p}(X)).
\]
\end{theorem}

%\textcolor{red}{\begin{theorem}\label{thm:PCA_stability1}
%Let $M$ be an $m-$dimensional submanifold of $\mathbb{R}^n$, $X$ be a finite $n-$generic subset and $\mathfrak{p}$ a $\delta$ perturbation for $\delta \in [0, \delta_0)$ then:
%\[
%\distance_b\big(\dgm(H(E^{\PCA}(X)))), \dgm(H(E^{\PCA}(\mathfrak{p}(X)))\big)
%\leq  C\delta = C\distance_H(X, \mathfrak{p}(X)). \]
%\end{theorem}}

%\textcolor{red}{\begin{theorem}[Standard Axes]
%Let $k, n\in \mathbb{N}$ with $k \ge n$, $X\subset\RR^n$ be a $k$-generic subset (Definition~\ref{def:genericity}), and $\mathfrak{p}\colon X\to \RR^n$ be a $\delta$-perturbation with $\delta \in [0, \delta_u(X))$ for $\delta_u(X)$ defined in Proposition~\ref{prop:stability_basismap}. Then
%\[
 %   \distance_b\!\big(\dgm(E^q(X))), \dgm(E^q(\mathfrak{p}(X))\big) \leq  Cq\diam(X)\delta %\le Cq\diam(X)\distance_H(X, \mathfrak{p}(X)),
%\]
%where $C$ is the constant from Lemma~\ref{prop:perturb_ell_intersec}.
%\end{theorem}}

The strategy of the proof is as in Section~\ref{sec:stability}: the first step is to prove that PCA ellipsoids filtrations of $X$ and $\mathfrak{p}$ are interleaved.
\begin{proposition}[Ellipsoids on Perturbed Data Intersect]\label{prop:PCA_perturb_ell_intersec}
    Let $X\subset \RR^n$ be a finite $n$-generic subset. Then there exists $\delta_0 > 0$ such that for every $x_1, x_2 \in X$ with 
    \[
        E^{\PCA}_\eps(x_1)\cap E^{\PCA}_\eps(x_2)\neq \emptyset,
    \]
    we have
    \[
        E^{\PCA}_{\eps+C\delta}({\mathfrak{p}(x_1)})\cap E^{\PCA}_{\eps+C\delta}(\mathfrak{p}(x_2))\neq \emptyset.
    \]
for all $\delta$-perturbations  \(\mathfrak{p}\colon X \to \RR^n\) with $\delta \in [0, \delta_0)$.
\end{proposition}
\begin{proof} We write 
\begin{align*}
\mathfrak{p}(x_i) = x_i + \delta p_i \text{ for some } p_i \in B_1(0).
\end{align*}
Suppose that
\begin{align*}
E^{\PCA}_\eps(x_1)\cap E^{\PCA}_\eps(x_2)\neq\emptyset .
\end{align*}
Hence there exists a point $x^{\ast}\in E^{\PCA}_\eps(x_1)\cap E^{\PCA}_\eps(x_2)$.
Let
\begin{align*}
     N_n^X(x_i)= \set{x_i^1,\dots ,x_i^n},\qquad i=1,2
\end{align*}
be the neighbourhood sets of $x_1$ and $x_2$ respectively. By Lemma \ref{lem:stability_neighborhoods} there exists a $\delta_0$ small enough such that for all $\delta \in [0, \delta_0)$ we have
\begin{align*}
    N_n^{\mathfrak{p}(X)}(\mathfrak{p}(x_i)) = \mathfrak{p}(N_n^X(x_i)) \quad \text{for }i=1,2.
\end{align*}
Hence, we can write
\begin{align*}
\mathfrak p(x_i^j) = x_i^j + \delta p_i^j\quad \text{for some } 
p_i^j\in B_1(0), i =1,2 \text{ and }j=1, \dots, n.
\end{align*}
We denote by $\overline{x_i}$ and $\overline{\mathfrak{p}(x_i)}$ the sample means of $N_n^X(x_i)$ and $N_n^{\mathfrak{p}(X)}(\mathfrak{p}(x_i))$ respectively.
Calculating $\overline{\mathfrak{p}(x_i)}$ explicitly yields:
\begin{align*}
\overline{\mathfrak{p}(x_i)} =\frac{1}{n}\sum_{j=1}^{n}\mathfrak p(x_i^j)
=\overline{x_i}+\delta\overline{{p}_i}, 
\end{align*}
where $\overline{p_i}$ denotes the mean of $\{p_i^1 \dots, p_i^\}$. Using this implies for neighbourhood matrices
\begin{align*}
    \mathbf{N}_n(\mathfrak{p}(x_i)) = \mathbf{N}_n(x_i) + \delta P_i,
\end{align*}
where $P_i$ is the $n\times n$-matrix whose $j$-th column is given by $p_i^j - \overline{p_i}$.
%where we define 
%\begin{align}
%  \mathfrak{p}(L_i) \coloneqq \begin{pmatrix}
%        | & | & | &  \\
%        \mathfrak{p}(x_1^i) - \overline{\mathfrak{p}(x^i)} & \cdots & \mathfrak{p}(x_n^i) - \overline{\mathfrak{p}(x^i)}\\
%        | & | & |
%    \end{pmatrix}.
%\end{align}
For brevity write $M_i = \mathbf{N}_n(x_i)$, $\tilde{M}_i = \mathbf{N}_n(\mathfrak{p}(x_i))$, and
\begin{align*}
A_i:=M_iP_i^T + P_iM_i^T\quad \text{and}\quad B_i = P_iP_i^T.
\end{align*}
Then
\begin{align*}
\tilde{M}_i\tilde{M}_i^T
=M_iM_i^T + \delta A_i + \delta^2 B_i.
\end{align*}
Choose $\delta_0$ small enough such that for all $\delta \in [0, \delta_0)$ we have
\begin{align}
\norm*{(M_iM_i^T)^{-1}\bigl(\delta A_i + \delta^2B_i\bigr)}<1
\qquad i=1,2.
\label{eq:small}
\end{align}
Because of~\eqref{eq:small} the Neumann series yields
\begin{align}
\begin{aligned}
\bigl(\tilde{M}_i\tilde{M}_i^T\bigr)^{-1}
&=\bigl(M_iM_i^T\bigr)^{-1}\Bigl[\bigl(I+\bigl(M_iM_i^T\bigr)^{-1}
(\delta A_i+\delta^2B_i)\bigr)\Bigr]^{-1}\\
&=\bigl(M_iM_i^T\bigr)^{-1}\sum_{k=0}^{\infty}\bigl[-\bigl(M_iM_i^T\bigr)^{-1}
(\delta A_i + \delta^2 B_i)\bigr]^{k}\\
& = \bigl(M_iM_i^T\bigr)^{-1}\Bigl[I - \delta\bigl(M_iM_i^T\bigr)^{-1} A_i +\mathcal{O}(\delta^2)\Bigr]
\end{aligned}
\label{eq:Neumann}
\end{align}
Write
\begin{align*}  
q_i(\delta):=(x^{\ast}-x_i-\delta p_i)^T \bigl(\tilde{M}_i\tilde{M}_i^T\bigr)^{-1} (x^{\ast} - x_i -\delta p_i),\qquad i=1,2 .
\end{align*}
At $\delta=0$ we have $q_i(0)\leq \eps$ because $x^{\ast}\in E^{\PCA}_\eps(x_i)$.  
Using~\eqref{eq:Neumann}  we obtain
\begin{align*}
    \begin{aligned}
        &q_i(\delta)= (x^*-p_i)^T(M_iM_i^T)^{-1}(x^*-p_i)  +\delta\Bigl( (x^*-p_i)^TA_i(M_iM_i^T)^{-2}(x^*-p_i) \\&-p_i^T(M_iM_i^T)^{-1}(x^*-p_i)- (x^*-p_i)^T(M_iM_i^T)^{-1}p_i\Bigl) +\mathcal{O}(\delta^2)
        \\& = q_i(0) + C \delta +\mathcal O(\delta^2) \quad(\delta\to 0),
    \end{aligned}
\end{align*}
for $ C = (x^*-p_i)^TA_i(M_iM_i^T)^{-2}(x^*-p_i) -p_i^T(M_iM_i^T)^{-1}(x^*-p_i)- (x^*-p_i)^T(M_iM_i^T)^{-1}p_i $.
Hence, there exists some $\delta_0$ small enough such that for every $\delta \in [0, \delta_0) $:
\[x^* \in E^{\PCA}_{\eps +C\delta}(\mathfrak{p}(x_1))\cap E^{\PCA}_{\eps +C\delta}(\mathfrak{p}(x_2)). \]
\medskip\noindent Hence, the claim follows.
\end{proof}
In the same way as in Section~\ref{sec:stability}, we use this to prove the interleaving property.
\begin{corollary}[PCA Ellipsoid interleaving]\label{cor:PCA_Ellipsoid_interleaving}
    Let $X$ be a finite $n$-generic subset of $\RR^n$. Then there exists a $\delta_0$ small enough such that for all $\delta\in [0,\delta_0)$ and for every $\delta$-perturbation $\mathfrak{p}\colon X\to \RR^n$, $E^{\PCA}(X)$ and $E^{\PCA}(\mathfrak{p}(X))$ are $C\cdot\delta$-interleaved.
\end{corollary}
\begin{proof}
Let $\mathfrak{p}$ be a $\delta$-perturbations.
and $\sigma$ be in $E^{\PCA}_\eps(X)$. By definition for all $x_1, x_2\in \sigma$ it holds:
\[E^{\PCA}_\eps(x_1) \cap E^{\PCA}_\eps(x_2)\neq \emptyset.\]
Thus by Proposition \ref{prop:PCA_perturb_ell_intersec} we know that there exists $\delta_0$ such that for each $\delta \in [0, \delta_0)$ it holds:
\[E^{\PCA}_{\eps+C\delta}(\mathfrak{p}(x_1))\cap E^{\PCA}_{\eps+C\delta}(\mathfrak{p}(x_1))\neq \emptyset.\]
This implies that $\mathfrak{p}(\sigma) \in E^{\PCA}_{\eps+C \delta}(\mathfrak{p}(X))$.
Due to symmetry, we get the same result for the inverse of $\mathfrak{p}$.
Hence, we have proved the claim.
\end{proof}
In the same way, this leads directly to the stability result.

\begin{proof}[Proof of Theorem~\ref{thm:PCA_stability}]
    Note that persistence modules arising from finite subsets via PCA ellipsoid construction are always $q$-tame. Hence, the Theorem is a direct application of Corollary \ref{cor:PCA_Ellipsoid_interleaving} and Theorem \ref{thm:Chazal}..
\end{proof}
\begin{remark}
    On the one hand, this proof is slightly more restrictive than in the case of Rips-type ellipsoids since it works only if the neighborhood size equals the dimension of the ambient space. On the other hand, we did not use the spectral gap assumption. One could modify the proof of Section~\ref{sec:stability} to this case if one were to swap the inverse with the Penrose pseudoinverse.
\end{remark}

\subsection{Experimental Results with PCA Ellipsoids}

The PCA axes ellipsoids are also implemented in the code. The construction process is again as described in Algorithm~\ref{alg:construct_ellipsoids}, except that, instead of fixed axes ratios, we use the axes ratios corresponding to the ratios of the eigenvalues coming from PCA.

\begin{figure}[h]
    \centering
    \includegraphics[width=0.8\textwidth]{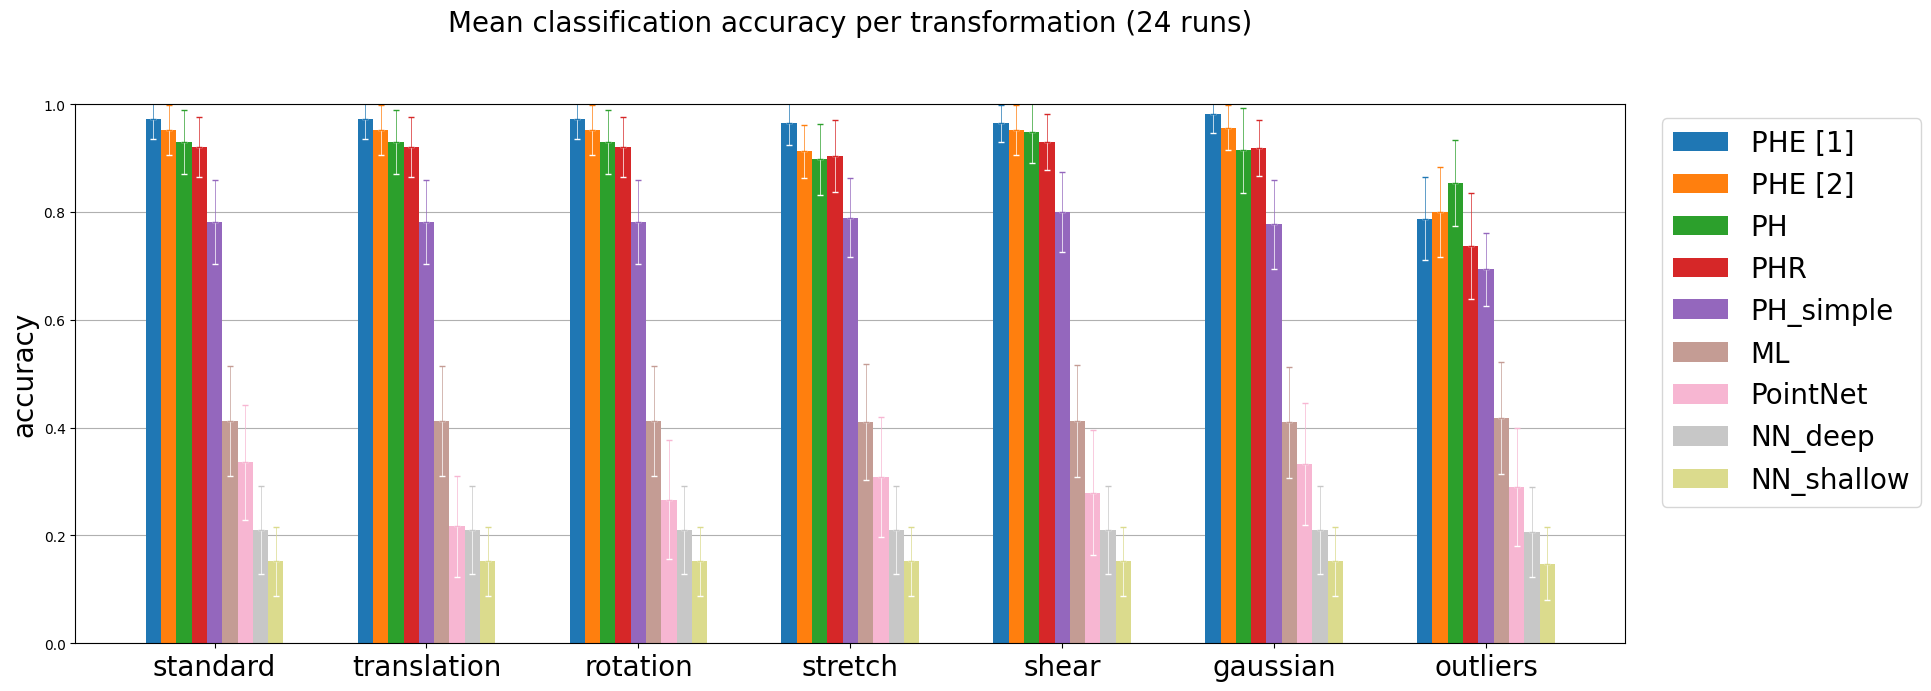}
    \caption{Classification accuracies across 24 runs on 100 point clouds, each consisting of 300 points. 
    PHE [1] refers to the pipeline using ellipsoid complexes with axes ratios $2:1$ and PCA neighbourhood size of 17.
    PHE [2] denotes the pipeline using ellipsoid complexes with PCA neighbourhood size of 25 and axes ratios corresponding to the ratios of eigenvalues of PCA. More details, as well as an explanation of other pipelines can be found in Section~\ref{subsec:point-cloud-classification}. 
    }
    \label{fig:point_cloud_classification_with_pca}
\end{figure}

In Figure~\ref{fig:point_cloud_classification_with_pca}, we show how ellipsoids with PCA axes perform in classification tasks, compared to other methods introduced in Section~\ref{subsec:point-cloud-classification}. In the figure, PHE [1] refers to Rips-type ellipsoid complexes with orientations determined by performing PCA on neighbourhoods of size 17 and with ellipsoid axes ratios $2:1$. PHE [2] refers to Rips-type ellipsoid complexes with orientations determined by performing PCA on neighbourhoods of size 25 and axes ratios coming from eigenvalues of the PCA. The remaining notation is the same as described in Section~\ref{subsec:point-cloud-classification}.

The values of the neighbourhood sizes, and in the case of PHE [1], the values of axes ratios, were selected because they performed best amongst all tested values.

As can be seen from Figure~\ref{fig:point_cloud_classification_with_pca}, ellipsoid complexes with PCA axes performed worse than ellipsoid complexes with fixed axes ratios. Nevertheless, the two ellipsoids-based methods performed better on average then all other methods.

\subsection{$k$-generic point clouds are open and dense}
Let $k, n, N$ be positive integers such that $N\geq k+1$ and $k \geq n$. Denote by $\mathcal{G}_{n,k}^N$ the set of all $N$ element subsets of $\R^n$ such that the $k$-neighborhood centered at each element of the subset is $k$-generic. We shall call an element of $\mathcal{G}_{n, k}^N$ a \define{$k$-generic point cloud with $N$ points in $\R^n$}. One may view $\mathcal{G}_{n, k}^N$ as a subset of $(\R^n)^N$ by assigning an arbitrary order to the elements in any subset contained in $\mathcal{G}_{n, k}^N$.
%Furthermore, for $N\in \mathbb{N}$ we define
%\[
%\mathcal{G}^N_{n,k} \coloneqq \underbrace{\mathcal{G}_{n, k}\times \cdots\times \mathcal{G}_{n, k}}_{N\text{ times}}.
%\]
%Intuitively, one should think of an element of $\mathcal{G}_{n, k}^N$ as the partition of a point cloud into $k$-neighborhoods.
%Note that $\mathcal{G}^N_{n,k}$ is a subset of $(\mathbb{R}^n)^N$. 
\begin{proposition}\label{prop:open_and_dense}
    The set of $k$-generic point clouds with $N$ points in $\mathbb{R}^n$ is open and dense in $(\mathbb{R}^n)^N$ endowed with the product Euclidean topology. In particular, any point cloud can be perturbed by an arbitrarily small amount to a $k$-generic point cloud.
\end{proposition}
\begin{proof}
First we prove that $\mathcal{G}^N_{n,k}$ is open in  $(\mathbb{R}^n)^N$. Let $X\in \mathcal{G}^N_{n,k}$ be arbitrary and write $X=(p_1,\dots,p_N)$ with $p_i\neq p_j$ for $i\neq j$.
Define
\begin{align*}
    \rho \coloneqq \min_{i\neq j}\|p_i-p_j\|>0 \quad\text{ and }\quad \varepsilon_0 \coloneqq \frac{\rho}{4}.
\end{align*}
For each $i\in\{1,\dots,N\}$, the separation condition implies that the numbers
$\{\|p_j-p_i\|: j\neq i\}$ are pairwise distinct. Order them as
\[
0<r_{i,1}<\cdots<r_{i,N-1},
\]
and set
\begin{align*}
    \Delta_i \coloneqq \min\Bigl(\min_{1\le a<b\le k}(r_{i,b}-r_{i,a}),\ r_{i,k+1}-r_{i,k}\Bigr)>0 \quad\text{ and }\quad \Delta \coloneqq \min_{1\le i\le N}\Delta_i>0
\end{align*}
Furthermore set $\varepsilon_1 \coloneqq \frac{\Delta}{8}$.
Moreover, since $X$ is $k$-generic (with $m$-gap), we have
\[
\eta_X \coloneqq \min_{1\le i\le N}\Bigl(\sigma_m(\mathbf N_k(p_i))-\sigma_{m+1}(\mathbf N_k(p_i))\Bigr)>0.
\]
We also set $\varepsilon_2\coloneqq \frac{\eta_X}{8\sqrt{k}}$ and $\varepsilon \coloneqq \min(\varepsilon_0,\varepsilon_1,\varepsilon_2).$
\newline
\newline
Let $Y=(q_1,\dots,q_N)$ satisfy $\max_{1\le i\le N}\|q_i-p_i\|<\varepsilon$.
Then for $i\neq j$ by the reverse triangle inequality
\begin{align*}
    \|q_i-q_j\|
    &\ge \|p_i-p_j\|-\|q_i-p_i\|-\|q_j-p_j\|
    \ge \rho-2\varepsilon
    \ge \frac{\rho}{2}>0,
\end{align*}
hence the points of $Y$ are pairwise distinct.
\newline
\newline
Fix $i\neq j $. By the reverse triangle inequality,
\begin{align} \label{eq:reverseTriangle}
\bigl|\|q_j-q_i\|-\|p_j-p_i\|\bigr|
\le \|q_j-p_j\|+\|q_i-p_i\|
<2\varepsilon.
\end{align}
Hence, for any $i \neq j, \ell$ using \ref{eq:reverseTriangle} twice implies:
\begin{align*}
   \|q_j-q_i\|-\|p_j-p_i\| + \|p_\ell-p_i\| - \|q_\ell-q_i\|
<4\varepsilon.
\end{align*}
Assuming that $\|p_\ell-p_i\|-\|p_j-p_i\|\ge 4\varepsilon$ implies:
\[
\|p_j-p_i\|<\|p_\ell-p_i\|
\ \Longrightarrow\
\|q_j-q_i\|<\|q_\ell-q_i\|.
\]
Since $4\varepsilon\le \Delta_i$, the strict ordering of the first $k$ distances from $p_i$
and the strict gap $r_{i,k}<r_{i,k+1}$ persist for $q_i$. Therefore, for each $i$, the set
$N_k(q_i)$ has exactly $k$ points and is strictly ordered by distance; in particular,
the neighbor indices of $q_i$ coincide with those of $p_i$.
\newline
\newline
Now fix $i$ and write $N_k(p_i)=\{p_{j_1},\dots,p_{j_k}\}$ (same indices for $q_i$).
Let $\bar p_i=\frac1k\sum_{\ell=1}^k p_{j_\ell}$ and $\bar q_i=\frac1k\sum_{\ell=1}^k q_{j_\ell}$.
Then $\|\bar q_i-\bar p_i\|\le \varepsilon$, and for each column $\ell$,
\[
\|(q_{j_\ell}-\bar q_i)-(p_{j_\ell}-\bar p_i)\|
\le \|q_{j_\ell}-p_{j_\ell}\|+\|\bar q_i-\bar p_i\|
<2\varepsilon.
\]
Hence by the Proposition \ref{prop:norm_comp} we have:
\[
\|\mathbf N_k(q_i)-\mathbf N_k(p_i)\|_F < 2\sqrt{k}\,\varepsilon.
\]
Using Corollary 7.3.5 of \cite{Horn_Johnson_1985}, we obtain for all $a$
\[
\bigl|\sigma_a(\mathbf N_k(q_i))-\sigma_a(\mathbf N_k(p_i))\bigr|
< 2\sqrt{k}\,\varepsilon.
\]
Therefore,
\begin{align*}
&\sigma_m(\mathbf N_k(q_i))-\sigma_{m+1}(\mathbf N_k(q_i))
\\&\ge \bigl(\sigma_m(\mathbf N_k(p_i))-\sigma_{m+1}(\mathbf N_k(p_i))\bigr)
      -\bigl|\sigma_m(\mathbf N_k(q_i))-\sigma_m(\mathbf N_k(p_i))\bigr|
      -\bigl|\sigma_{m+1}(\mathbf N_k(q_i))-\sigma_{m+1}(\mathbf N_k(p_i))\bigr| \\
&> \eta_X - 4\sqrt{k}\,\varepsilon
\ \ge\ \frac{\eta_X}{2},
\end{align*}
since $|\sigma_a(\mathbf N_k(q_i))-\sigma_a(\mathbf N_k(p_i))|<2\sqrt{k}\varepsilon$ for all $a$ and
$\varepsilon\le \varepsilon_2=\eta_X/(8\sqrt{k})$.
Thus $Y$ satisfies the $m$-spectral gap condition (with uniform constant $\eta_X/2$), and consequently
$Y\in \mathcal{G}^N_{n,k}$. This shows that $\mathcal{G}^N_{n,k}$ is open.

Now we argue that $\mathcal{G}^N_{n,k}$ is dense in $(\RR^n)^N$. For $1\le i<j\le N$ we define
\[
F_{i,j}(X)\coloneqq \|p_i-p_j\|^2,
\]
and for $1\le i\le N$ and $j,\ell\in\{1,\dots,N\}\setminus\{i\}$, $j<\ell$, set
\[
G_{i;j,\ell}(X)\coloneqq \|p_j-p_i\|^2-\|p_\ell-p_i\|^2 .
\]
Furthermore, for $1\le i\le N$ and any subset $I=\{j_1,\dots,j_k\}\subset\{1,\dots,N\}\setminus\{i\}$ of cardinality $k$ we define
\[
\bar p_I \coloneqq \frac1k\sum_{t=1}^k p_{j_t},\qquad
\mathbf N_I(p_i)\coloneqq \begin{pmatrix} \,|& &|\\ p_{j_1}-\bar p_I&\cdots&p_{j_k}-\bar p_I\\ |& &| \end{pmatrix}\in\mathbb R^{d\times k},
\]
and its Gram matrix $H_{i,I}(X)\coloneqq \mathbf N_I(p_i)^\top \mathbf N_I(p_i)\in\mathbb R^{k\times k}$.
Let
\[
\chi_{i,I}(\lambda;X)\coloneqq \det(\lambda I_k - H_{i,I}(X))
\]
and define
\[
D_{i,I}(X)\coloneqq \mathrm{Disc}\bigl(\chi_{i,I}(\cdot;X)\bigr),
\]
the discriminant of $\chi_{i,I}$. Hence, $D_{i,I}(X)=0$ if and only if $H_{i,I}(X)$ has a repeated eigenvalue, equivalently, if $\mathbf N_I(p_i)$ has a repeated
singular value.

Define
\[
\mathcal U \coloneqq (\mathbb R^n)^N \setminus
\Biggl(
\bigcup_{i<j}\{F_{i,j}=0\}\ \cup\
\bigcup_{i}\ \bigcup_{j<\ell}\{G_{i;j,\ell}=0\}\ \cup\
\bigcup_{i}\ \bigcup_{I}\{D_{i,I}=0\}
\Biggr),
\]
where in the middle union $j,\ell$ range over $\{1,\dots,N\}\setminus\{i\}$ and in the last union $I$ ranges over
all $k$-subsets of $\{1,\dots,N\}\setminus\{i\}$. Note that trivially $\mathcal{U}\subset \mathcal{G}^N_{n,k}$.
\newline
\newline
Each set $\{F_{i,j}=0\}$ and $\{G_{i;j,\ell}=0\}$ is the zero set of a nonzero polynomial.
Moreover, for each $(i,I)$, $D_{i,I}$ is not the zero polynomial, hence $\{D_{i,I}=0\}$ is a proper algebraic subset.
Therefore the union above is a finite union of proper algebraic sets, so $\mathcal U$ is open and dense in
$(\mathbb R^n)^N$, thus also $\mathcal{G}^N_{n,k}$.

\end{proof}

\end{document}
